# Supplementary material for: Manekko: Training Small but Foundational 3D Medical Models by Mimicking Natural Vision Model Features
Source: arXiv:2611.37538 source file (2026-11-27)
Supplement: Supplementary file 1 [file supplementary.tex]

\documentclass[10pt,twocolumn,letterpaper]{article}

% Supplementary material, compiled separately from main.tex.
% Each section lives in its own file under suppl/.

\usepackage[review]{cvpr}      % To produce the REVIEW version

\input{preamble}

\definecolor{cvprblue}{rgb}{0.21,0.49,0.74}
% Cross-references to the main paper (needs main.aux: compile main.tex first).
\usepackage[pagebackref,breaklinks,colorlinks,allcolors=cvprblue]{hyperref}
\usepackage{zref-xr}
\zxrsetup{toltxlabel}
\zexternaldocument*{main}

\def\paperID{*****}
\def\confName{CVPR}
\def\confYear{2027}

\title{Manekko: Unreasonable Effectiveness of Copying Features}

\author{Puru Vaish \and Christoph Brune \and Jelmer M. Wolterink \\
University of Twente \\
{\tt\small \{p.vaish,c.brune,j.m.wolterink\}@utwente.nl}
}

% Keep numbering distinct from the main paper.
\renewcommand{\thesection}{\Alph{section}}
\renewcommand{\thefigure}{S\arabic{figure}}
\renewcommand{\thetable}{S\arabic{table}}
\renewcommand{\theequation}{S\arabic{equation}}

\begin{document}

\maketitlesupplementary
\input{suppl/A_implementation}
\input{suppl/B_datasets}
\input{suppl/C_evaluation}
\input{suppl/C2_finetuning_duration}
\input{suppl/D_full_results}
\input{suppl/E_sensitivity}
\input{suppl/F_reference_models}
\input{suppl/G_feature_analysis}
% \input{suppl/H_qualitative}
\input{suppl/I_pancancer}
\input{suppl/J_limitations}
\input{suppl/K_ranking_reloaded}

{
    \small
    \bibliographystyle{ieeenat_fullname}
    \bibliography{main}
}

\end{document}
