# Supplementary material for: Manekko: Training Small but Foundational 3D Medical Models by Mimicking Natural Vision Model Features
Source: arXiv:2611.37538 source file (2026-11-27)
Supplement: Supplementary file 2 [file supp_memory.tex]

\small
\setlength{\tabcolsep}{4pt}
\begin{tabular}{l c cc}
    \toprule
    & \textbf{Params (M)} & \multicolumn{2}{c}{\textbf{Memory (GiB)}} \\
    \cmidrule(lr){2-2}\cmidrule(lr){3-4}
    Encoder & Enc.\ + Dec. & Peak & Fwd.\ extra \\
    \midrule
    \rowcolor{oursrow}
    \ours                             & 74.9  & 4.17 & 4.05 \\
    Primus-M                          & 163.0 & 4.72 & 4.12 \\
    3DINO~\cite{3dino}                & 334.9 & 5.28 & 4.02 \\
    nnFoundation~\cite{nnfoundation}  & 558.5 & 6.29 & 4.15 \\
    \bottomrule
\end{tabular}
